# Supplementary material for: Valley-selective optical Stark effect probed by Kerr rotation
Source: arXiv:1710.09739 ancillary file (2017-10-26)
Supplement: Supplementary file 1 [file LaMountain2017_SupplementaryMaterial.pdf]

# Supplementary Material: Valley-Selective Optical Stark Effect Probed by Kerr Rotation

Trevor LaMountain[1], Hadallia Bergeron[2], Itamar Balla[2], Teodor K. Stanev[3], Mark C. Hersam[1,2,4,5], and Nathaniel P. Stern[1,3]

[1] *Applied Physics Program, Northwestern University, Evanston, Illinois 60208, USA*
[2] *Department of Materials Science and Engineering, Northwestern University, Evanston, Illinois 60208, USA*
[3] *Department of Physics and Astronomy, Northwestern University, Evanston, Illinois 60208, USA*
[4] *Department of Chemistry, Northwestern University, Evanston, Illinois 60208, USA*
[5] *Department of Electrical Engineering and Computer Science, Northwestern University, Evanston, Illinois 60208, USA*

October 22, 2017

## 1. Experimental details

### 1.1. Time-resolved experiment setup

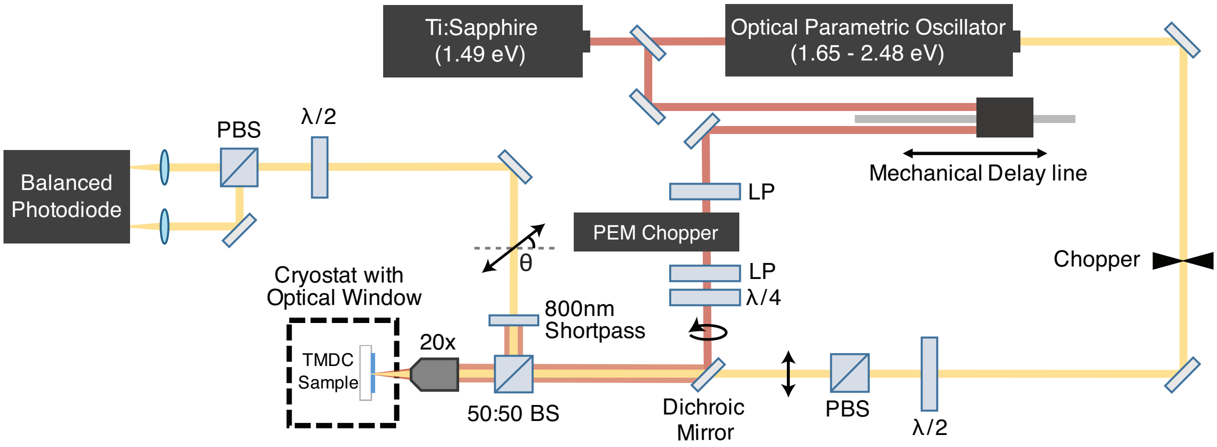


**Figure S1:** Schematic of the optics used in the TR-KR measurement.

## 1.2. $MoS_2$ sample preparation by chemical vapor deposition

Monolayer $MoS_2$ crystals were prepared using chemical vapor deposition directly on $SiO_2$/Si using a previously reported procedure [1]. Briefly, an $SiO_2$/Si substrate was placed in a 1 inch diameter quartz tube in the middle of a Lindberg/Blue furnace hot zone. An alumina boat containing 15 mg of $MoO_3$ powder was placed directly upstream of the substrate and an alumina boat containing 150 mg of sulfur power was placed 30 cm upstream of the $MoO_3$ (outside of the furnace). Preceding growth, an argon gas purging procedure and a bake-out at 150 °C are performed to remove contaminants and moisture. The growth was conducted at a pressure of 200 Torr with an Ar flow rate of 25 sccm. The furnace is heated to 800 °C while the sulfur was heated to 150 °C using a heating belt. These temperatures were maintained for 20 minutes, followed by natural cooling. Monolayer $WSe_2$ flakes were obtained by exfoliation as described in the Appendix A of the main text.

## 1.3. Monolayer $WSe_2$ characterization

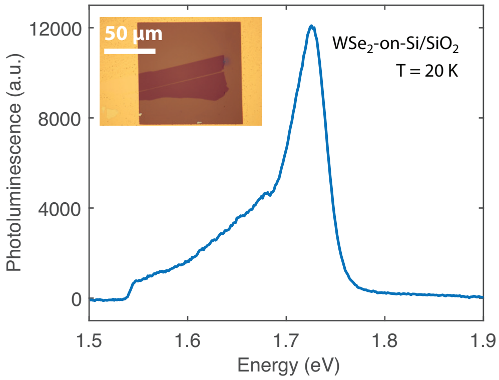


**Figure S2:** Photoluminescence of $WSe_2$ sample reported in main document at 20 K. Inset: Optical image of sample, showing monolayer flake and gold alignment window.

# 2. Extraction of pulse width from transient Kerr rotation signal

Temporal pump-probe measurements of the Stark shift only have signal near $t = 0$ when pump and probe pulses overlap (Fig. S3). The width of this signal originates in the laser pulses and the dynamics of the level renormalization of the Stark shift, and should be wider than the nominal pulsewidth of the laser itself. Here, we provide details of the observed signal widths.

The pulse width $\Delta t$ of the ultrafast Ti:Sapphire laser used in the experiments is defined as the full-width half-maximum of the pulse envelope, which is assumed to be Gaussian for simplicity. Since both pump and probe pulses are derived from the same laser, we assume

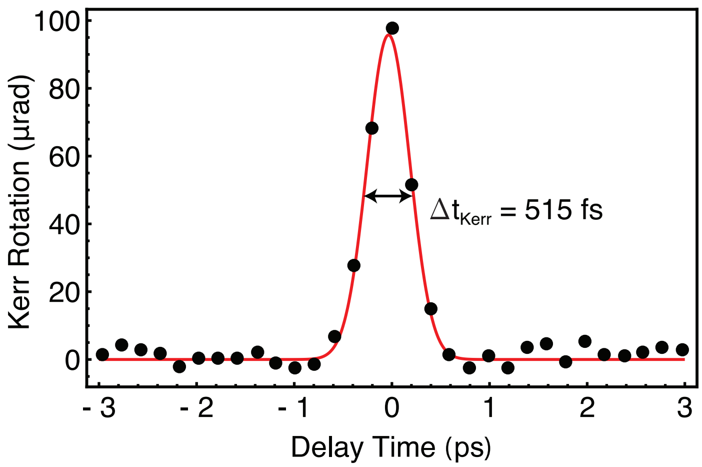


**Figure S3:** Typical gaussian fit to TR-KR data. Pulse width of the pump and probe pulses $\Delta t = \frac{1}{\sqrt{2}}\Delta t_{\text{Kerr}}$.

that they have the same pulse width. The pulse width is extracted from the transient Kerr rotation signal $\theta(t)$ induced by the valley-selective optical Stark effect. The instantaneous $\theta(t)$ is a function of pump-probe delay time $t$ and directly proportional to both the pump intensity ($I_{\text{pump}}$), which induces the rotation, and the probe intensity ($I_{\text{probe}}$), which measures the rotation. The experimentally measured Kerr angle is proportional to the overlap of these two beam profiles.

$$\theta(t) = C\int_{-\infty}^{\infty} I_{pump}(t-t')I_{probe}(t')dt' \tag{S1}$$

where $C$ is a proportionality constant and

$$\begin{aligned} I_{\text{pump}}(t') &= A_1 e^{\frac{-4\ln 2\, t'^2}{\Delta t^2}} \\ I_{\text{probe}}(t') &= A_2 e^{\frac{-4\ln 2\, t'^2}{\Delta t^2}} \end{aligned} \tag{S2}$$

where $A_1$ and $A_2$ are the peak intensities of the respective Gaussian pulses. This is a standard convolution integral with a Gaussian solution of

$$\theta(t) = CA_1A_2\sqrt{\frac{\pi\Delta t^2}{8ln(2)}}e^{\frac{-4ln(2)t^2}{2\Delta t^2}}. \tag{S3}$$

Therefore, the measured Kerr angle $\theta(t)$ has a full-width half-maximum $\Delta t_{\text{Kerr}} = \sqrt{2}\Delta t$.

Measured across multiple transient Kerr signals, $\Delta t_{\text{Kerr}} = 530 \pm 40$ fs from which we extract a pulse width $\Delta t = 380 \pm 30$ fs. The approximation of identical Gaussian pulse widths for pump and probe ignores the nominally longer pulse width of the OPO probe compared to the Ti:sapphire pump or any nonlinearities in conversion of pump-induced $\Delta E$ into $\theta$ or $\Delta R$ signals. Moreover, we do not have sufficient knowledge of the Stark shift dynamics to precisely understand their influence on the observed signal widths. This analysis simply provides a representative characterization of the observed pulse width for estimating fluence rather than a definitive measurement of the laser pulses.

# 3. Extraction of dielectric function from Lorentz oscillator model

All samples consist of a TMDC monolayer on a Si/$SiO_2$ substrate. Following the analysis of Ref. [2], we use a thin-film model to extract the dielectric function of the TMDC monolayer from measurements of the combined flake-substrate system. In the case of $WSe_2$, the system is treated as three distinct layers: a semi-infinite Si substrate, a $SiO_2$ layer of thickness $d_{\mathrm{SiO_2}}$, and a TMDC of thickness $d_{\mathrm{WSe_2}}$ with an interface to air. At normal incidence, the reflectance $R$ of the sample is the magnitude squared of the field reflection coefficient $r$, which is found from the Fresnel equations for the three-interface system:

$$R = |r|^2 = \left| \frac{r_1 e^{-i(\beta_1+\beta_2)} + r_2 e^{i(\beta_1-\beta_2)} + r_3 e^{i(\beta_1+\beta_2)} + r_1 r_2 r_3 e^{-i(\beta_1-\beta_2)}}{e^{-i(\beta_1+\beta_2)} + r_1 r_2 e^{i(\beta_1-\beta_2)} + r_1 r_3 e^{i(\beta_1+\beta_2)} + r_2 r_3 e^{-i(\beta_1-\beta_2)}} \right|^2 \tag{S4}$$

with

$$\begin{aligned} r_1 &= \frac{\tilde{n}_{\mathrm{air}} - \tilde{n}_{\mathrm{WSe_2}}}{\tilde{n}_{\mathrm{air}} + \tilde{n}_{\mathrm{WSe_2}}}, \quad r_2 = \frac{\tilde{n}_{\mathrm{WSe_2}} - \tilde{n}_{\mathrm{SiO_2}}}{\tilde{n}_{\mathrm{WSe_2}} + \tilde{n}_{\mathrm{SiO_2}}}, \quad r_3 = \frac{\tilde{n}_{\mathrm{SiO_2}} - \tilde{n}_{\mathrm{Si}}}{\tilde{n}_{\mathrm{SiO_2}} + \tilde{n}_{\mathrm{Si}}}, \\ \beta_1 &= 2\pi \frac{\tilde{n}_{\mathrm{WSe_2}} d_{\mathrm{WSe_2}}}{\lambda}, \quad \beta_2 = 2\pi \frac{\tilde{n}_{\mathrm{SiO_2}} d_{\mathrm{SiO_2}}}{\lambda} \end{aligned} \tag{S5}$$

where $\lambda$ is the wavelength of the light in vacuum, $d_{\mathrm{WSe_2}} = 0.65$ nm and $d_{\mathrm{SiO_2}} = 285 \pm 5$ nm are the material thicknesses, and $\tilde{n}_j = n_j + ik_j$ is the complex index of refraction for material $j$.

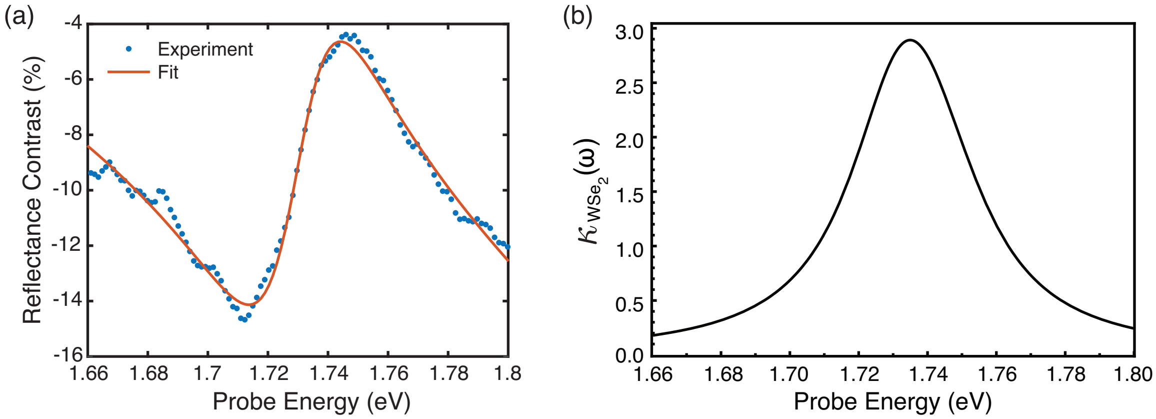


**Figure S4:** (a) Reflectance contrast spectrum of $WSe_2$ with no pump near the A exciton. The red curve is a fit to $R_{\mathrm{contrast}}$ using the Lorentz oscillator model. (b) Imaginary refractive index $\kappa_{\mathrm{WSe_2}}$ extracted from $R_{\mathrm{contrast}}$ in (a).

The refractive index of $WSe_2$ in the region of the A exciton is modeled by a single Lorentz oscillator at the exciton resonance plus four additional oscillators centered at higher energies to account for off-resonance contributions. The reflectance spectrum of the bare substrate $R_{\mathrm{bg}}$ is obtained by setting $n_{\mathrm{WSe_2}} = 1$, which is used to define the reflection contrast spectrum $R_{\mathrm{contrast}} = (R - R_{\mathrm{bg}})/R_{\mathrm{bg}}$. We use this model to fit the experimental $R_{\mathrm{contrast}}$

spectrum without the pump beam to determine the unperturbed parameters for the Lorentz oscillator model (Fig. S4). We allow $d_{\mathrm{WSe}_2}$ to vary within ±5 nm to account for uncertainty in the oxide thickness. We then use these oscillator parameters to fit the $\Delta R/R$ spectrum induced by the pump by allowing the central energy and width of the A exciton oscillator to vary, while holding all other parameters fixed. We account for the finite width of the probe by convoluting a normalized Gaussian (FWHM= 10 meV) with the $\Delta R/R$ spectrum predicted by the model when fitting the measured $\Delta R/R$ data. This allows extraction of the pump-induced blue shift $\Delta E$ in the exciton energy caused by the optical Stark effect. This procedure follows the approach of Ref. [2], with extension to the Kerr rotation angle.

# 4. Uncertainty in $\Delta E$ extracted from fits

The uncertainty in $\Delta E$ extracted from the fits to the $\theta$ and $\Delta R/R$ spectra has two primary contributions: the uncertainty in the measured $\theta$ and $\Delta R/R$ ($\sigma_m$), and the uncertainty in the unperturbed oscillator parameters found by fitting the $R_{\mathrm{contrast}}$ spectrum ($\sigma_p$). We quantify $\sigma_m$ using a bootstrapping method. We fit the measured data set $(x_i, y_i)$ to the model. A new set of synthetic data $(x_i, y_i^*)$ is generated by adding random values to the model prediction such that $y_i^* = y_i^{\mathrm{model}} + \epsilon$ where $\epsilon$ is normally distributed around 0 with standard deviation inherited from the experimental random uncertainty in the measured data. We then fit this synthetic data and repeat this process 100 times. The standard deviation of the set of extracted $\Delta E$ is used to estimate $\sigma_m$. To estimate $\sigma_p$, we fit 5 different $R_{\mathrm{contrast}}$ spectra measured at the same point on the sample to extract 5 distinct sets of unperturbed oscillator parameters. We then fit the $\Delta R/R$ and $\theta$ spectra using each of these 5 unperturbed parameter sets, which gives a distribution of values for $\Delta E$. The standard deviation of this $\Delta E$ distribution is used to estimate $\sigma_p$. We estimate the total uncertainty by adding $\sigma_m$ and $\sigma_p$ in quadrature: $\sigma_{\mathrm{total}} = \sqrt{\sigma_m^2 + \sigma_m^2}$. The 95% confidence intervals are estimated by $\pm 2 \times \sigma_{\mathrm{total}}$. For the Kerr rotation measurement, $\sigma_p > \sigma_m$. If the initial oscillator parameters were well-knowm $\sigma_p$ could be ignored, causing the confidence interval to drop to ±1.4 ueV. By contrast, ignoring $\sigma_p$ for the TR-R analysis yields a confidence interval of ±8.5 ueV. This highlights the markedly more precise estimation of $\Delta E$ from the TR-KR measurement due to the lower measurement uncertainty.

# 5. Reflectance and Kerr rotation sensitivity to the refractive index

Figure S5a shows how the $\Delta R/R$ and Kerr rotation ($\theta$) spectra induced by the optical Stark effect correspond to the real and imaginary parts of the refractive index of $\mathrm{WSe}_2$. For the reflective $\mathrm{Si/SiO}_2$ substrate we used in our measurements, the $\theta$ spectrum tracks the $\Delta\kappa$ spectrum and the $\Delta R/R$ spectrum is similar to $\Delta n$. The converse is true for a transparent sapphire substrate. While the lineshapes all agree qualitatively, there are some quantitative

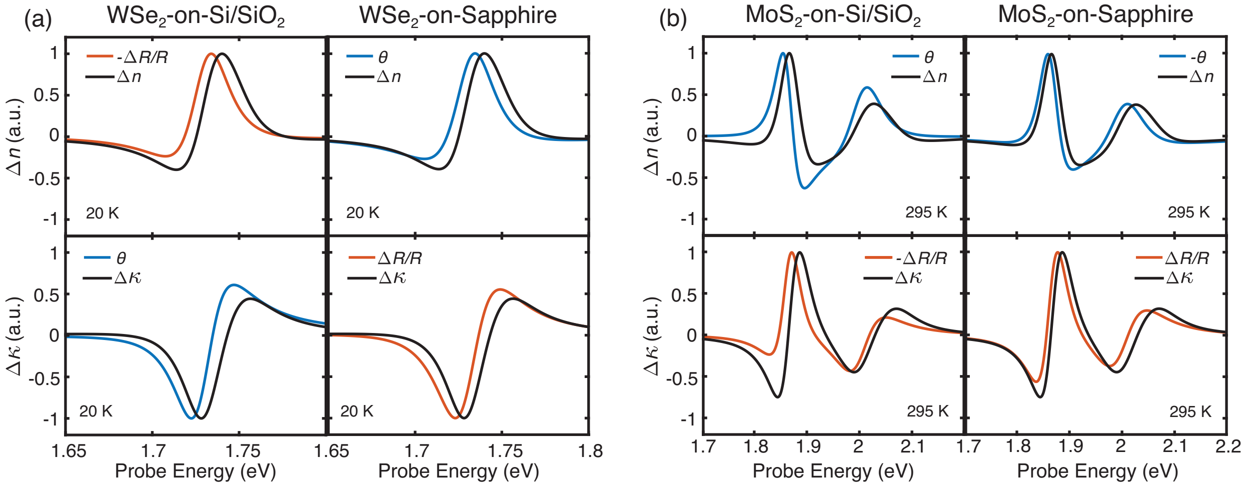


**Figure S5:** Simulations of $\theta$ and $\Delta R/R$ spectra induced by the optical Stark effect for $WSe_2$ and $MoS_2$ on reflective and transparent substrates. The unperturbed refractive index of each TMDC is the same for all simulations (found from fit to $R_{\text{contrast}}$). The spectra are normalized for ease of comparison. (a) For $WSe_2$, the $\Delta R/R$ and Kerr rotation spectra correspond to opposite parts of the refractive index for transparent and reflective substrates. (b) In the case of $MoS_2$, the $\Delta R/R$ and Kerr rotation spectra roughly correspond to the same parts of the refractive index for both substrates. The larger discrepancy in the case of the Si/$SiO_2$ substrate is due to thin-film effects.

discrepancies due to the influence of the multiple layers in the Fresnel equations, such as the locations of zeros and the sign of the Kerr and $\Delta R/R$ spectra relative to $\Delta\kappa$ and $\Delta n$. Still, the agreement between spectral features of the measured quantities and the induced $\Delta\tilde{n}_{\text{WSe}_2}(\omega)$ spectra demonstrates how each measurement is primarily sensitive to complementary parts of the refractive index.

In the case of transparent substrates with minimal thin-film effects, $\theta$ tracks $\Delta\kappa$ and $\Delta R/R$ tracks $\Delta n$. However, for standard reflective substrates like Si/$SiO_2$, the relationship is more complicated. In our experiments, we find that Kerr rotation probes $\Delta\kappa$ in $WSe_2$-on-Si/$SiO_2$ ($d_{\text{SiO}_2}$ = 285 nm) but for $MoS_2$-on-Si/$SiO_2$ ($d_{\text{SiO}_2}$ = 320 nm) Kerr rotation probes $\Delta n$ (Figure S5b). This can be understood by considering the influence of thin-film effects. Due to thin-film interference, the reflectance spectrum of the TMDC-substrate system can be sensitive to both the real and imaginary parts of $\tilde{n}_{\text{TMDC}}(\omega)$, depending on the thickness of the oxide layer and the particular energy dependence of $\tilde{n}_{\text{TMDC}}(\omega)$. In our measurements, the $R_{\text{contrast}}$ spectrum for $WSe_2$-on-Si/$SiO_2$ shows a feature at the A exciton energy that mimics $n_{\text{WSe}_2}(\omega)$ (Figure S4a), while the $R_{\text{contrast}}$ spectrum for $MoS_2$-on-Si/$SiO_2$ mimics $\kappa_{\text{MoS}_2}(\omega)$ near the A and B exciton resonances (Main document Fig. 4b). Consequently, $\Delta R/R$ corresponds to $\Delta n$ in $WSe_2$ and $\Delta\kappa$ in $MoS_2$. Since $\Delta R/R$ and Kerr rotation probe complementary parts of the refractive index, the correspondence between $\Delta n$ and Kerr rotation in $MoS_2$ is expected.

# 6. Supplemental data

## 6.1. Comparison of modulation schemes

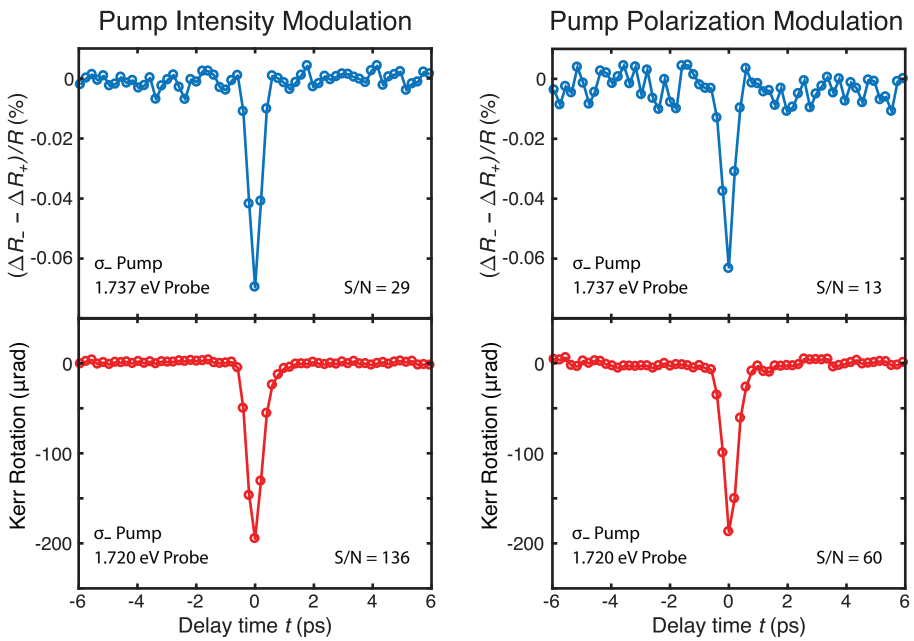


**Figure S6:** Time-resolved measurements of $WSe_2$ at 20K using different pump modulation schemes. The probe energy corresponds to the peak signal for both the Kerr rotation and reflectance measurements. All measurements use the same lock-in amplifier time constant for comparison. (Left column) TR-R and TR-KR using a PEM chopper to modulate pump intensity. In this scheme, two separate measurements using $\sigma_-$ and $\sigma_+$ probe polarizations are subtracted to find the TR-R signal induced by the Stark shift $(\Delta R_- - \Delta R_+)/R$. (Right column) TR-R and TR-KR using a PEM to modulate pump polarization between $\sigma_-$ and $\sigma_+$. A lock-in amplifier referenced to the polarization modulation frequency directly detects $(\Delta R_- - \Delta R_+)/R$ in a single measurement. For Kerr rotation, this scheme measures the difference between $\theta$ induced by a $\sigma_-$ and $\sigma_+$ pump. Since $\theta$ is equal in magnitude but opposite in sign for the two pump helicities, this measurement detects twice the signal $(2\theta)$ of the intensity-modulated scheme (scaled out here for comparison). For the conditions of these measurements, the intensity-modulated schemes have superior signal-to-noise (S/N). In all cases, S/N can be improved with longer averaging time constant.

## 6.2. Comparison between multiple $WSe_2$ samples

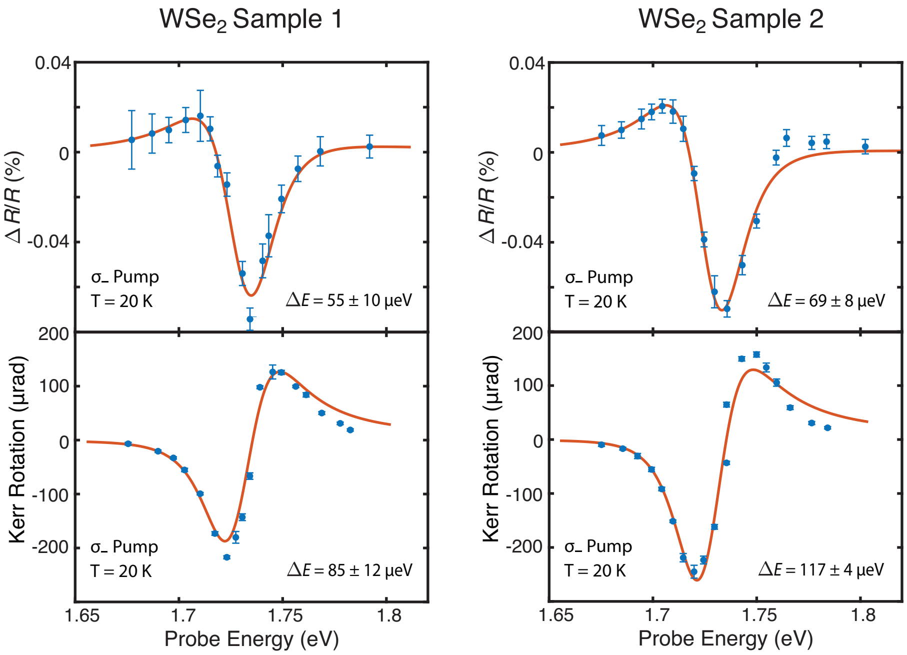


**Figure S7:** TR-R and TR-KR spectra from two additional $WSe_2$ samples on $Si/SiO_2$ substrates. For both of these measurements the TR-KR spectrum was measured first, then a quarter-wave plate (QWP) was inserted in the probe path to generate circularly-polarized probe light necessary for the TR-R measurement. However, the introduction of the QWP led to a slight change in the overlap of the pump and probe spots between the two measurements, resulting in a disagreement in the extracted $\Delta E$. The measurements presented in the main document keep the probe QWP in place for both measurements, which significantly reduces the discrepancy.

## 6.3. Data from $MoS_2$

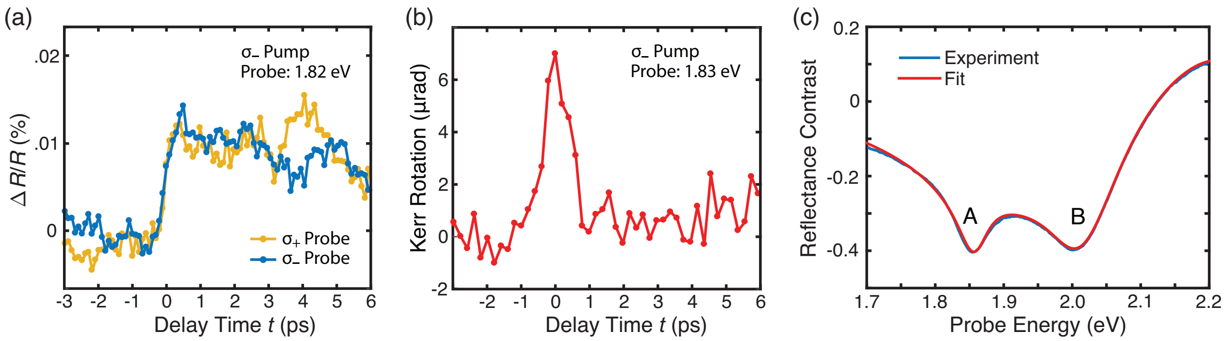


**Figure S8:** Time-resolved measurements of $MoS_2$. (a) $\Delta R/R$ for 1.82 eV probe dominated by background signal. There is no discernable asymmetry between $\sigma_+$ and $\sigma_-$ probes attributable to the Stark effect. (b) Kerr rotation for 1.83 eV probe showing a clear signal at $t \sim 0$. (c) Reflectance contrast spectrum for $MoS_2$ on $Si/SiO_2$ substrate at 295 K showing A and B exciton features at 1.85 eV and 2.0 eV, respectively.

# References


[1] Shastry, T. A. *et al.* Mutual photoluminescence quenching and photovoltaic effect in large-area single-layer $MoS_2$–polymer heterojunctions. *ACS Nano* **10**, 10573–10579 (2016).

[2] Ye, Z., Sun, D. & Heinz, T. F. Optical manipulation of valley pseudospin. *Nat. Phys.* (2016).
